# Supplementary material for: Angle-adjustable density field formulation for modeling crystalline microstructures
Source: arXiv:1805.06022 source file (2018-05-15)
Supplement: Supplementary file 1 [file angle_pfc_supp.pdf]

# Supplemental Material
# Angle-Adjustable Density Field Formulation for Modeling Crystalline Microstructures


Zi-Le Wang,[1] Zhirong Liu,[1,*] and Zhi-Feng Huang[2,†]

[1] College of Chemistry and Molecular Engineering, Peking University, Beijing 100871, China
[2] Department of Physics and Astronomy, Wayne State University, Detroit, Michigan 48201, USA


## I. DERIVATION OF ANGLE-DEPENDENT FREE ENERGY FUNCTIONAL WITH ROTATIONAL INVARIANCE

As shown in Eq. (1) of the main text, the free energy functional in classical density functional theory is written as

$$\Delta F/k_BT = \rho_0 \int d\mathbf{r}(1+n)\ln(1+n) - \sum_m \frac{1}{m!}\rho_0^m \int \prod_{j=1}^{m} d\mathbf{r}_j \; C^{(m)}(\mathbf{r}_1, \mathbf{r}_2, ..., \mathbf{r}_m) n(\mathbf{r}_1) n(\mathbf{r}_2) \cdots n(\mathbf{r}_m), \tag{S1}$$

where the first term is the ideal-gas entropy contribution, and $n = (\rho - \rho_0)/\rho_0$ is the atomic-number-density variation field, with $\rho_0$ a reference-state density. Without losing generality, the $m$-point direct correlation function is of the form $C^{(m)}(\mathbf{r}_1, \mathbf{r}_2, ..., \mathbf{r}_m) = C^{(m)}(\mathbf{r}_1 - \mathbf{r}_2, \mathbf{r}_1 - \mathbf{r}_3, ..., \mathbf{r}_1 - \mathbf{r}_m)$, given that there are only $m-1$ independent spatial coordinates for $C^{(m)}$. Its Fourier transform in dimension $n_d$ is given by

$$C^{(m)}(\mathbf{r}_1, \mathbf{r}_2, ..., \mathbf{r}_m) = \frac{1}{(2\pi)^{(m-1)n_d}} \int d\mathbf{q}_1 d\mathbf{q}_2 ... d\mathbf{q}_{m-1} \hat{C}^{(m)}(\mathbf{q}_1, \mathbf{q}_2, ..., \mathbf{q}_{m-1}) e^{i\mathbf{q}_1\cdot(\mathbf{r}_1-\mathbf{r}_2)} e^{i\mathbf{q}_2\cdot(\mathbf{r}_1-\mathbf{r}_3)} ... e^{i\mathbf{q}_{m-1}\cdot(\mathbf{r}_1-\mathbf{r}_m)}. \tag{S2}$$

Substituting it into the integrals in Eq. (S1), we have

$$\begin{aligned}
&(2\pi)^{(m-1)n_d} \int \prod_{j=1}^{m} d\mathbf{r}_j C^{(m)}(\mathbf{r}_1, \mathbf{r}_2, ..., \mathbf{r}_m) n(\mathbf{r}_1) n(\mathbf{r}_2) \cdots n(\mathbf{r}_m) \\
&= \int d\mathbf{r}_1 n(\mathbf{r}_1) \int d\mathbf{q}_1 d\mathbf{q}_2 ... d\mathbf{q}_{m-1} e^{i\mathbf{q}_1\cdot\mathbf{r}_1} e^{i\mathbf{q}_2\cdot\mathbf{r}_1} ... e^{i\mathbf{q}_{m-1}\cdot\mathbf{r}_1} \hat{C}^{(m)}(\mathbf{q}_1, \mathbf{q}_2, ..., \mathbf{q}_{m-1}) \\
&\quad \times \left[\int d\mathbf{r}_2 n(\mathbf{r}_2) e^{-i\mathbf{q}_1\cdot\mathbf{r}_2}\right] \left[\int d\mathbf{r}_3 n(\mathbf{r}_3) e^{-i\mathbf{q}_2\cdot\mathbf{r}_3}\right] ... \left[\int d\mathbf{r}_m n(\mathbf{r}_m) e^{-i\mathbf{q}_{m-1}\cdot\mathbf{r}_m}\right] \\
&= \int d\mathbf{r} n(\mathbf{r}) \int d\mathbf{q}_1 d\mathbf{q}_2 ... d\mathbf{q}_{m-1} e^{i\mathbf{q}_1\cdot\mathbf{r}} e^{i\mathbf{q}_2\cdot\mathbf{r}} ... e^{i\mathbf{q}_{m-1}\cdot\mathbf{r}} \hat{C}^{(m)}(\mathbf{q}_1, \mathbf{q}_2, ..., \mathbf{q}_{m-1}) \hat{n}(\mathbf{q}_1)\hat{n}(\mathbf{q}_2)...\hat{n}(\mathbf{q}_{m-1}).
\end{aligned} \tag{S3}$$

Specifically, for three- and four-point direct correlation functions,

$$\int d\mathbf{r}_1 d\mathbf{r}_2 d\mathbf{r}_3 C^{(3)}(\mathbf{r}_1, \mathbf{r}_2, \mathbf{r}_3) n(\mathbf{r}_1) n(\mathbf{r}_2) n(\mathbf{r}_3) = \frac{1}{(2\pi)^{2n_d}} \int d\mathbf{r} n(\mathbf{r}) \int d\mathbf{q}_1 d\mathbf{q}_2 e^{i\mathbf{q}_1\cdot\mathbf{r}} e^{i\mathbf{q}_2\cdot\mathbf{r}} \hat{n}(\mathbf{q}_1)\hat{n}(\mathbf{q}_2) \hat{C}^{(3)}(\mathbf{q}_1, \mathbf{q}_2), \tag{S4}$$

$$\begin{aligned}
&\int d\mathbf{r}_1 d\mathbf{r}_2 d\mathbf{r}_3 d\mathbf{r}_4 C^{(4)}(\mathbf{r}_1, \mathbf{r}_2, \mathbf{r}_3, \mathbf{r}_4) n(\mathbf{r}_1) n(\mathbf{r}_2) n(\mathbf{r}_3) n(\mathbf{r}_4) \\
&\qquad = \frac{1}{(2\pi)^{3n_d}} \int d\mathbf{r} n(\mathbf{r}) \int d\mathbf{q}_1 d\mathbf{q}_2 d\mathbf{q}_3 e^{i\mathbf{q}_1\cdot\mathbf{r}} e^{i\mathbf{q}_2\cdot\mathbf{r}} e^{i\mathbf{q}_3\cdot\mathbf{r}} \hat{n}(\mathbf{q}_1)\hat{n}(\mathbf{q}_2)\hat{n}(\mathbf{q}_3) \hat{C}^{(4)}(\mathbf{q}_1, \mathbf{q}_2, \mathbf{q}_3),
\end{aligned} \tag{S5}$$

which will be used in the following derivation.

### Three-point correlation $C^{(3)}$

From Eq. (2) of the main text obtained from the property of isotropic Cartesian tensors [1], the general rotationally invariant expansion form of $\hat{C}^{(3)}(\mathbf{q}_1, \mathbf{q}_2)$ is given by

$$\begin{aligned}
\hat{C}^{(3)}(\mathbf{q}_1, \mathbf{q}_2) = \hat{C}_0^{(3)} + \sum_{M=1}^{\infty} \Bigg[ & \hat{C}_1^{(3)} q_1^{2M} + \hat{C}_2^{(3)} q_2^{2M} + \sum_{\mu=1}^{M-1} \hat{C}_{2\mu,2M-2\mu}^{(3)} q_1^{2\mu} q_2^{2M-2\mu} \\
& + \sum_{\mu=0}^{M-1} \sum_{\nu=0}^{M-1-\mu} \hat{C}_{2\mu,2\nu,2M-2\mu-2\nu}^{(3)} q_1^{2\mu} q_2^{2\nu} (\mathbf{q}_1\cdot\mathbf{q}_2)^{M-\mu-\nu} \Bigg].
\end{aligned} \tag{S6}$$

Using Eq. (S4) we get the following transformation of $\hat{C}^{(3)}$ terms

$$q_{1(2)}^{2M} \to (-1)^M \int d\mathbf{r} n^2 \nabla^{2M} n, \qquad q_1^{2\mu} q_2^{2M-2\mu} \to (-1)^M \int d\mathbf{r} n (\nabla^{2\mu} n)(\nabla^{2M-2\mu} n). \tag{S7}$$

Also noting that

$$\mathbf{q}_j \cdot \mathbf{q}_k = \frac{1}{2}\left(|\mathbf{q}_j + \mathbf{q}_k|^2 - q_j^2 - q_k^2\right), \tag{S8}$$

we have (for $\eta = M - \mu - \nu$)

$$\begin{aligned}
q_1^{2\mu} q_2^{2\nu} (\mathbf{q}_1 \cdot \mathbf{q}_2)^\eta \to & \frac{1}{(2\pi)^{2d}} \int d\mathbf{r} n \int d\mathbf{q}_1 d\mathbf{q}_2 e^{i(\mathbf{q}_1+\mathbf{q}_2)\cdot\mathbf{r}} \hat{n}(\mathbf{q}_1)\hat{n}(\mathbf{q}_2) \frac{1}{2^\eta} \left(|\mathbf{q}_1 + \mathbf{q}_2|^2 - q_1^2 - q_2^2\right)^\eta q_1^{2\mu} q_2^{2\nu} \\
= & \frac{1}{(2\pi)^{2d}} \int d\mathbf{r} n \int d\mathbf{q}_1 d\mathbf{q}_2 e^{i(\mathbf{q}_1+\mathbf{q}_2)\cdot\mathbf{r}} \hat{n}(\mathbf{q}_1)\hat{n}(\mathbf{q}_2) \\
& \times \frac{1}{2^\eta} \sum_{u=0}^{\eta} \binom{\eta}{u} |\mathbf{q}_1 + \mathbf{q}_2|^{2u} (-1)^{\eta-u} \sum_{w=0}^{\eta-u} \binom{\eta-u}{w} q_1^{2w+2\mu} q_2^{2\eta-2u-2w+2\nu} \\
= & \frac{1}{2^\eta} \sum_{u=0}^{\eta} \sum_{w=0}^{\eta-u} (-1)^{\eta-u} \binom{\eta}{u} \binom{\eta-u}{w} \int d\mathbf{r} n \frac{1}{(2\pi)^{2d}} \\
& \times (-\nabla^2)^u \left[ \int d\mathbf{q}_1 d\mathbf{q}_2 e^{i(\mathbf{q}_1+\mathbf{q}_2)\cdot\mathbf{r}} q_1^{2w+2\mu} q_2^{2\eta-2u-2w+2\nu} \hat{n}(\mathbf{q}_1)\hat{n}(\mathbf{q}_2) \right] \\
= & \frac{1}{2^\eta} \sum_{u=0}^{\eta} \sum_{w=0}^{\eta-u} (-1)^{\eta-u} \binom{\eta}{u} \binom{\eta-u}{w} \int d\mathbf{r} n \frac{1}{(2\pi)^{2d}} \\
& \times (-\nabla^2)^u \left\{ (-\nabla^2)^{w+\mu} \left[ \int d\mathbf{q}_1 e^{i\mathbf{q}_1\cdot\mathbf{r}} \hat{n}(\mathbf{q}_1) \right] (-\nabla^2)^{\eta-u-w+\nu} \left[ \int d\mathbf{q}_2 e^{i\mathbf{q}_2\cdot\mathbf{r}} \hat{n}(\mathbf{q}_2) \right] \right\} \\
= & \frac{1}{2^\eta} \sum_{u=0}^{\eta} \sum_{w=0}^{\eta-u} (-1)^{\mu+\nu-u} \binom{\eta}{u} \binom{\eta-u}{w} \int d\mathbf{r} \nabla^{2u} \left[ \left(\nabla^{2w+2\mu} n\right) \left(\nabla^{2\eta-2u-2w+2\nu} n\right) \right] \\
= & \frac{1}{2^\eta} \sum_{u=0}^{\eta} \sum_{w=0}^{\eta-u} (-1)^{\mu+\nu-u} \binom{\eta}{u} \binom{\eta-u}{w} \int d\mathbf{r} \left(\nabla^{2u} n\right) \left(\nabla^{2w+2\mu} n\right) \left(\nabla^{2\eta-2u-2w+2\nu} n\right).
\end{aligned} \tag{S9}$$

When $u = M$ or $u = 0$, the above formula gives the same term $n^2\nabla^{2M}n$ or $n(\nabla^{2\mu}n)(\nabla^{2M-2\mu}n)$ as that in Eq. (S7). Thus the free energy contribution from three-point direct correlation function can be written as (for all orders of $q$)

$$\begin{aligned}
\Delta\mathcal{F}^{(3)} = & \int d\mathbf{r} \left[ -\frac{1}{3} D_0 n^3 + \sum_{M=1}^{\infty} \sum_{\mu=0}^{M} \sum_{\nu=0}^{M-\mu} D_{\mu,\nu,M-\mu-\nu} \left(\nabla^{2\mu} n\right) \left(\nabla^{2\nu} n\right) \left(\nabla^{2M-2\mu-2\nu} n\right) \right] \\
= & \int d\mathbf{r} \left\{ -\frac{1}{3} D_0 n^3 + \sum_{M=1}^{\infty} \left[ D_M n^2 \nabla^{2M} n + \sum_{\mu=1}^{M-1} D_{\mu,M-\mu} n (\nabla^{2\mu} n)(\nabla^{2M-2\mu} n) \right. \right. \\
& \left. \left. + \sum_{\mu=1}^{M-1} \sum_{\nu=1}^{M-1-\mu} D_{\mu,\nu,M-\mu-\nu} \left(\nabla^{2\mu} n\right) \left(\nabla^{2\nu} n\right) \left(\nabla^{2M-2\mu-2\nu} n\right) \right] \right\}.
\end{aligned} \tag{S10}$$

To be more specific, the free energy terms at each order $\mathcal{O}(q^{2M})$ are given by

$$\begin{aligned}
& M = 1, \mathcal{O}(q^2) : D_1 n^2 \nabla^2 n, \\
& M = 2, \mathcal{O}(q^4) : D_2 n^2 \nabla^4 n + D_{11} n (\nabla^2 n)^2, \\
& M = 3, \mathcal{O}(q^6) : D_3 n^2 \nabla^6 n + D_{12} n (\nabla^2 n)(\nabla^4 n) + D_{111} (\nabla^2 n)^3, \\
& M = 4, \mathcal{O}(q^8) : D_4 n^2 \nabla^8 n + D_{13} n (\nabla^2 n)(\nabla^6 n) + D_{22} n (\nabla^4 n)^2 + D_{112} (\nabla^2 n)^2 (\nabla^4 n), \\
& M = 5, \mathcal{O}(q^{10}) : D_5 n^2 \nabla^{10} n + D_{14} n (\nabla^2 n)(\nabla^8 n) + D_{23} n (\nabla^4 n)(\nabla^6 n) + D_{113} (\nabla^2 n)^2 (\nabla^6 n) + D_{122} (\nabla^2 n)(\nabla^4 n)^2, \\
& \cdots\cdots
\end{aligned} \tag{S11}$$

It is important to note that any of the above free energy terms contributed by the $C^{(3)}$ expansion are angle-independent and isotropic. (An exception would be some infinite series of $\hat{C}^{(3)}(\mathbf{q}_1, \mathbf{q}_2)$ combining infinite orders of $q$ and corresponding to some special functions [2, 3], with more details given below in Sec. III.) This lack of angle dependency can be also illustrated through the expansion of the density field $n$ in terms of amplitudes $A_j(\mathbf{q}_j)$ for the reciprocal lattice vectors $\mathbf{q}_j$, i.e.,

$$n = n_0 + \sum_j A_j e^{i\mathbf{q}_j\cdot\mathbf{r}}, \qquad A_{-j}(-\mathbf{q}_j) = A_j^*(\mathbf{q}_j). \tag{S12}$$

Substituting it into the free energy functional Eq. (S10), we have (for a system of volume $V$)

$$\begin{aligned}
&\frac{1}{V}\int d\mathbf{r} n^3 = n_0^3 + 3n_0\sum_j |A_j|^2 + \sum_{jkl} A_j A_k A_l \delta_{\mathbf{q}_j+\mathbf{q}_k+\mathbf{q}_l,0},\\
&\frac{1}{V}\int d\mathbf{r} n^2\nabla^{2M} n = (-1)^M 2n_0 \sum_j q_j^{2M}|A_j|^2 + (-1)^M\sum_{jkl} q_j^{2M} A_j A_k A_l \delta_{\mathbf{q}_j+\mathbf{q}_k+\mathbf{q}_l,0},\\
&\frac{1}{V}\int d\mathbf{r} n(\nabla^{2\mu} n)(\nabla^{2M-2\mu} n) = (-1)^M n_0 \sum_j q_j^{2M}|A_j|^2 + (-1)^M\sum_{jkl} q_j^{2\mu} q_k^{2M-2\mu} A_j A_k A_l \delta_{\mathbf{q}_j+\mathbf{q}_k+\mathbf{q}_l,0},\\
&\frac{1}{V}\int d\mathbf{r}\left(\nabla^{2\mu} n\right)\left(\nabla^{2\nu} n\right)\left(\nabla^{2M-2\mu-2\nu} n\right) = (-1)^M\sum_{jkl} q_j^{2\mu} q_k^{2\nu} q_l^{2M-2\mu-2\nu} A_j A_k A_l \delta_{\mathbf{q}_j+\mathbf{q}_k+\mathbf{q}_l,0},
\end{aligned} \tag{S13}$$

all of which depend only on the lengths of $\mathbf{q}_j$ but not the angles between them.

### Four-point correlation $C^{(4)}$

The results for $C^{(4)}$ are much more complicated, although the derivation procedure is similar. The general expansion form of $\hat{C}^{(4)}(\mathbf{q}_1, \mathbf{q}_2, \mathbf{q}_3)$ is given by

$$\begin{aligned}
\hat{C}^{(4)}(\mathbf{q}_1, \mathbf{q}_2, \mathbf{q}_3) =& \hat{C}_0^{(4)} + \sum_{M=1}^{\infty}\left\{\sum_{j=1}^{3}\hat{C}_j^{(4)} q_j^{2M} + \sum_{\mu=0}^{M-1}\sum_{\nu=0}^{M-1-\mu}\hat{C}^{(4)}_{2\mu,2\nu,2M-2\mu-2\nu} q_1^{2\mu} q_2^{2\nu} q_3^{2M-2\mu-2\nu}\right.\\
&\left. + \sum_{\mu\nu\omega\kappa\tau}\hat{C}^{(4)}_{2\mu,2\nu,2\omega,\kappa,\tau} q_1^{2\mu} q_2^{2\nu} q_3^{2\omega}(\mathbf{q}_1\cdot\mathbf{q}_2)^{\kappa}(\mathbf{q}_2\cdot\mathbf{q}_3)^{\tau}(\mathbf{q}_3\cdot\mathbf{q}_1)^{M-\mu-\nu-\omega-\kappa-\tau}\right\}\\
&+ \sum_{\mu\nu\omega\kappa\tau\lambda}\hat{C}^{(4)}_{2\mu,2\nu,2\omega,\kappa,\tau,\lambda} q_1^{2\mu} q_2^{2\nu} q_3^{2\omega}(\mathbf{q}_1\cdot\mathbf{q}_2)^{\kappa}(\mathbf{q}_2\cdot\mathbf{q}_3)^{\tau}(\mathbf{q}_3\cdot\mathbf{q}_1)^{\lambda}\left[(\mathbf{q}_1\times\mathbf{q}_2)\cdot\mathbf{q}_3\right].
\end{aligned} \tag{S14}$$

Note that there is only 1 factor $(\mathbf{q}_1\times\mathbf{q}_2)\cdot\mathbf{q}_3$ in the expansion, instead of $[(\mathbf{q}_1\times\mathbf{q}_2)\cdot\mathbf{q}_3]^{\zeta}$ with power $\zeta \geq 2$, given that $[(\mathbf{q}_1\times\mathbf{q}_2)\cdot\mathbf{q}_3]^{\zeta} = (\sum_{\alpha\beta\gamma}\epsilon_{\alpha\beta\gamma} q_{1\alpha} q_{2\beta} q_{3\gamma})^{\zeta}$ and $\epsilon_{\alpha_1\beta_1\gamma_1}\epsilon_{\alpha_2\beta_2\gamma_2} = \delta_{\alpha_1\alpha_2}\delta_{\beta_1\beta_2}\delta_{\gamma_1\gamma_2} + \delta_{\alpha_1\beta_2}\delta_{\beta_1\gamma_2}\delta_{\gamma_1\alpha_2} + \delta_{\alpha_1\gamma_2}\delta_{\beta_1\alpha_2}\delta_{\gamma_1\beta_2} - \delta_{\alpha_1\alpha_2}\delta_{\beta_1\gamma_2}\delta_{\gamma_1\beta_2} - \delta_{\alpha_1\beta_2}\delta_{\beta_1\alpha_2}\delta_{\gamma_1\gamma_2} - \delta_{\alpha_1\gamma_2}\delta_{\beta_1\beta_2}\delta_{\gamma_1\alpha_2}$. Using Eqs. (S5) and (S8) we can derive the free energy contribution from four-point correlation as (for all orders of $q$)

$$\begin{aligned}
\Delta\mathcal{F}^{(4)} = \int d\mathbf{r}\Bigg\{&\frac{1}{4}E_0 n^4 + \sum_{M=1}^{\infty}\sum_{\mu\nu\omega\kappa\tau=0}^{M} E_{\mu\nu\omega\kappa\tau}\sum_{\alpha_{i'},\beta_{j'}=x,y,z}\left[\nabla^{2\mu}\left(n\nabla^{2\omega}\prod_{i'=1}^{\kappa}\prod_{j'=1}^{\tau}\partial_{\alpha_{i'}}\partial_{\beta_{j'}} n\right)\right]\\
&\times\left(\nabla^{2\nu}\prod_{i'=1}^{\kappa}\partial_{\alpha_{i'}} n\right)\left(\nabla^{2M-2\mu-2\nu-2\omega-2\kappa-2\tau}\prod_{j'=1}^{\tau}\partial_{\beta_{j'}} n\right)\\
&+ \sum_{\mu\nu\omega\kappa\tau\lambda} E_{\mu\nu\omega\kappa\tau\lambda}\, n\sum_{\alpha_{i'},\beta_{j'},\gamma_{k'}=x,y,z}\ \sum_{\alpha,\beta,\gamma=x,y,z}\epsilon_{\alpha\beta\gamma}\left(\nabla^{2\mu}\prod_{i'=1}^{\kappa}\prod_{k'=1}^{\lambda}\partial_{\alpha_{i'}}\partial_{\gamma_{k'}}\partial_{\alpha} n\right)\\
&\times\left(\nabla^{2\nu}\prod_{i'=1}^{\kappa}\prod_{j'=1}^{\tau}\partial_{\alpha_{i'}}\partial_{\beta_{j'}}\partial_{\beta} n\right)\left(\nabla^{2\omega}\prod_{j'=1}^{\tau}\prod_{k'=1}^{\lambda}\partial_{\beta_{j'}}\partial_{\gamma_{k'}}\partial_{\gamma} n\right)\Bigg\}
\end{aligned}$$

$$
\begin{aligned}
&= \int d\mathbf{r} \left\{ \frac{1}{4} E_0 n^4 + \sum_{M=1}^{\infty} \left\{ E_{0M} n^3 \nabla^{2M} n + \sum_{\mu=1}^{M-1} E_{0,\mu,M-\mu} n^2 (\nabla^{2\mu} n)(\nabla^{2M-2\mu} n) \right. \right. \\
&\quad + \sum_{\mu=1}^{M-1} \sum_{\nu=1}^{M-1-\mu} E_{0,\mu,\nu,M-\mu-\nu} n (\nabla^{2\mu} n)(\nabla^{2\nu} n)(\nabla^{2M-2\mu-2\nu} n) + E_M n^2 \nabla^{2M} n^2 \\
&\quad + \sum_{\mu=1}^{M-1} E_{\mu,M-\mu} n (\nabla^{2\mu} n^2)(\nabla^{2M-2\mu} n) + \sum_{\mu=1}^{M-1} \sum_{\nu=1}^{M-1-\mu} E_{\mu,\nu,M-\mu-\nu} (\nabla^{2\mu} n^2)(\nabla^{2\nu} n)(\nabla^{2M-2\mu-2\nu} n) \\
&\quad + \sum_{\mu=1}^{M-1} \sum_{\nu=0}^{M-1-\mu} \sum_{\omega=1}^{M-1-\mu-\nu} E_{\mu,\omega,\nu,M-\mu-\omega-\nu} \left[ \nabla^{2\mu} (n \nabla^{2\omega} n) \right] (\nabla^{2\nu} n)(\nabla^{2M-2\mu-2\nu-2\omega} n) \\
&\quad + \sum_{\mu\nu\omega\kappa\tau=0}^{M-1} E_{\mu\nu\omega\kappa\tau} \sum_{\alpha_{i'},\beta_{j'}=x,y,z} \left[ \nabla^{2\mu} \left( n \nabla^{2\omega} \prod_{i'=1}^{\kappa} \prod_{j'=1}^{\tau} \partial_{\alpha_{i'}} \partial_{\beta_{j'}} n \right) \right] \\
&\qquad \left. \times \left( \nabla^{2\nu} \prod_{i'=1}^{\kappa} \partial_{\alpha_{i'}} n \right) \left( \nabla^{2M-2\mu-2\nu-2\omega-2\kappa-2\tau} \prod_{j'=1}^{\tau} \partial_{\beta_{j'}} n \right) \right\} \\
&\quad + \sum_{\mu\nu\omega\kappa\tau\lambda} E_{\mu\nu\omega\kappa\tau\lambda}\, n \sum_{\alpha_{i'},\beta_{j'},\gamma_{k'}=x,y,z} \sum_{\alpha,\beta,\gamma=x,y,z} \epsilon_{\alpha\beta\gamma} \left( \nabla^{2\mu} \prod_{i'=1}^{\kappa} \prod_{k'=1}^{\lambda} \partial_{\alpha_{i'}} \partial_{\gamma_{k'}} \partial_\alpha n \right) \\
&\qquad \left. \times \left( \nabla^{2\nu} \prod_{i'=1}^{\kappa} \prod_{j'=1}^{\tau} \partial_{\alpha_{i'}} \partial_{\beta_{j'}} \partial_\beta n \right) \left( \nabla^{2\omega} \prod_{j'=1}^{\tau} \prod_{k'=1}^{\lambda} \partial_{\beta_{j'}} \partial_{\gamma_{k'}} \partial_\gamma n \right) \right\}. \qquad \text{(S15)}
\end{aligned}
$$

Many terms here can be reduced via integration by parts over a unit cell. The factor $\epsilon_{\alpha\beta\gamma}$ in the last set of terms is from $(\mathbf{q}_1 \times \mathbf{q}_2) \cdot \mathbf{q}_3 = \sum_{\alpha\beta\gamma} \epsilon_{\alpha\beta\gamma} q_{1\alpha} q_{2\beta} q_{3\gamma}$. These terms correspond to odd order of $q$ expansion of $\hat{C}^{(4)}$, and are given by

$$
\begin{aligned}
&\int d\mathbf{r} n \sum_{\alpha,\beta,\gamma=x,y,z} \epsilon_{\alpha\beta\gamma} \left( \nabla^{2\mu} \prod_{i'=1}^{\kappa} \prod_{k'=1}^{\lambda} \partial_{\alpha_{i'}} \partial_{\gamma_{k'}} \partial_\alpha n \right) \left( \nabla^{2\nu} \prod_{i'=1}^{\kappa} \prod_{j'=1}^{\tau} \partial_{\alpha_{i'}} \partial_{\beta_{j'}} \partial_\beta n \right) \left( \nabla^{2\omega} \prod_{j'=1}^{\tau} \prod_{k'=1}^{\lambda} \partial_{\beta_{j'}} \partial_{\gamma_{k'}} \partial_\gamma n \right) \\
&= \int d\mathbf{r} n \begin{vmatrix}
\nabla^{2\mu} \prod_{i'=1}^{\kappa} \prod_{k'=1}^{\lambda} \partial_{\alpha_{i'}} \partial_{\gamma_{k'}} \partial_x n & \nabla^{2\nu} \prod_{i'=1}^{\kappa} \prod_{j'=1}^{\tau} \partial_{\alpha_{i'}} \partial_{\beta_{j'}} \partial_x n & \nabla^{2\omega} \prod_{j'=1}^{\tau} \prod_{k'=1}^{\lambda} \partial_{\beta_{j'}} \partial_{\gamma_{k'}} \partial_x n \\
\nabla^{2\mu} \prod_{i'=1}^{\kappa} \prod_{k'=1}^{\lambda} \partial_{\alpha_{i'}} \partial_{\gamma_{k'}} \partial_y n & \nabla^{2\nu} \prod_{i'=1}^{\kappa} \prod_{j'=1}^{\tau} \partial_{\alpha_{i'}} \partial_{\beta_{j'}} \partial_y n & \nabla^{2\omega} \prod_{j'=1}^{\tau} \prod_{k'=1}^{\lambda} \partial_{\beta_{j'}} \partial_{\gamma_{k'}} \partial_y n \\
\nabla^{2\mu} \prod_{i'=1}^{\kappa} \prod_{k'=1}^{\lambda} \partial_{\alpha_{i'}} \partial_{\gamma_{k'}} \partial_z n & \nabla^{2\nu} \prod_{i'=1}^{\kappa} \prod_{j'=1}^{\tau} \partial_{\alpha_{i'}} \partial_{\beta_{j'}} \partial_z n & \nabla^{2\omega} \prod_{j'=1}^{\tau} \prod_{k'=1}^{\lambda} \partial_{\beta_{j'}} \partial_{\gamma_{k'}} \partial_z n
\end{vmatrix} \qquad \text{(S16)}
\end{aligned}
$$

The determinant is equal to 0 when at least two of $\mu, \nu, \omega$ are equal to each other and at least two of $\kappa, \tau, \lambda$ are 0.

Some examples of different $q$ orders are listed in the following:

$$
\begin{aligned}
&\mathcal{O}(q^2) : n^3 \nabla^2 n, n^2 \nabla^2 n^2 \qquad \rightarrow \quad n^3 \nabla^2 n \quad \text{(after integrating over a unit cell)} \\
&\mathcal{O}(q^3) : (\mathbf{q}_1 \times \mathbf{q}_2) \cdot \mathbf{q}_3 \text{ in } q \text{ expansion, with } \mu = \nu = \omega = \kappa = \tau = \lambda = 0 \qquad \rightarrow \quad 0 \\
&\mathcal{O}(q^4) : n^3 \nabla^4 n, n^2 \nabla^4 n^2, n^2 (\nabla^2 n)^2, n(\nabla^2 n)(\nabla^2 n^2), n(\boldsymbol{\nabla} n) \cdot [\nabla^2 (n \boldsymbol{\nabla} n)] \\
&\qquad \rightarrow \quad n^3 \nabla^4 n, n^2 \nabla^4 n^2, n^2 (\nabla^2 n)^2 \quad \text{(after integrating over a unit cell)} \\
&\mathcal{O}(q^5) : q_j^2 (\mathbf{q}_1 \times \mathbf{q}_2) \cdot \mathbf{q}_3, (\mathbf{q}_j \cdot \mathbf{q}_k)(\mathbf{q}_1 \times \mathbf{q}_2) \cdot \mathbf{q}_3 \text{ in } q \text{ expansion} \qquad \rightarrow \quad 0 \\
&\cdots\cdots \qquad \text{(S17)}
\end{aligned}
$$

Note that at $\mathcal{O}(q^4)$ the only angle-dependent term is $n^2 \nabla^4 n^2$, which has been used in previous studies of 2D square pattern formation [4]. Another $\mathcal{O}(q^4)$ nonlinear gradient term studied previously [5], $|\nabla n|^4$, is of similar effect given that $\int d\mathbf{r} |\nabla n|^4 = \int d\mathbf{r} (n^2 \nabla^4 n^2 / 4 - n^3 \nabla^4 n / 3)$ over a unit cell.

There are totally 5 types of $\Delta \mathcal{F}^{(4)}$ terms in Eq. (S15), two of which, $n^4$ and $n(\nabla^{2\mu} n)(\nabla^{2\nu} n)(\nabla^{2M-2\mu-2\nu} n)$ (with integers $\mu, \nu \geq 0$, $M \geq \mu + \nu$), are angle independent. Expanding the density field $n$ in terms of amplitudes $A_j$ and

wave vectors $\mathbf{q}_j$ as in Eq. (S12), they can be written as

$$\frac{1}{V}\int d\mathbf{r}n^4 = n_0^4 + 6n_0^2\sum_j |A_j|^2 + 4n_0\sum_{jkl} A_jA_kA_l\delta_{\mathbf{q}_j+\mathbf{q}_k+\mathbf{q}_l,0} + \sum_{ijkl} A_iA_jA_kA_l\delta_{\mathbf{q}_i+\mathbf{q}_j+\mathbf{q}_k+\mathbf{q}_l,0}, \tag{S18}$$

$$\frac{1}{V}\int d\mathbf{r}n(\nabla^{2\mu}n)(\nabla^{2\nu}n)(\nabla^{2M-2\mu-2\nu}n) = (-1)^M \left[ n_0\sum_{jkl} q_j^{2\mu}q_k^{2\nu}q_l^{2M-2\mu-2\nu}A_jA_kA_l\delta_{\mathbf{q}_j+\mathbf{q}_k+\mathbf{q}_l,0} + \sum_{ijkl} q_j^{2\mu}q_k^{2\nu}q_l^{2M-2\mu-2\nu}A_iA_jA_kA_l\delta_{\mathbf{q}_i+\mathbf{q}_j+\mathbf{q}_k+\mathbf{q}_l,0}\right]. \tag{S19}$$

For the other 3 types of angle dependent terms,

$$\begin{aligned}&\frac{1}{V}\int d\mathbf{r}\left[\nabla^{2\mu}(n\nabla^{2\omega}n)\right](\nabla^{2\nu}n)(\nabla^{2M-2\mu-2\nu-2\omega}n)\Big|_{\mu\geq1,\nu,\omega\geq0,M\geq\mu+\nu+\omega}\\ &= (-1)^M\left[n_0\sum_{jkl} q_j^{2\mu+2\omega}q_k^{2\nu}q_l^{2M-2\mu-2\nu-2\omega}A_jA_kA_l\delta_{\mathbf{q}_j+\mathbf{q}_k+\mathbf{q}_l,0}\right.\\ &\qquad\left.+\sum_{ijkl}|\mathbf{q}_i+\mathbf{q}_j|^{2\mu}q_j^{2\omega}q_k^{2\nu}q_l^{2M-2\mu-2\nu-2\omega}A_iA_jA_kA_l\delta_{\mathbf{q}_i+\mathbf{q}_j+\mathbf{q}_k+\mathbf{q}_l,0}\right],\end{aligned} \tag{S20}$$

$$\begin{aligned}&\frac{1}{V}\int d\mathbf{r}\sum_{\alpha_{i'},\beta_{j'}=x,y,z}\left[\nabla^{2\mu}\left(n\nabla^{2\omega}\prod_{i'=1}^{\kappa}\prod_{j'=1}^{\tau}\partial_{\alpha_{i'}}\partial_{\beta_{j'}}n\right)\right]\left(\nabla^{2\nu}\prod_{i'=1}^{\kappa}\partial_{\alpha_{i'}}n\right)\left(\nabla^{2M-2\mu-2\nu-2\omega-2\kappa-2\tau}\prod_{j'=1}^{\tau}\partial_{\beta_{j'}}n\right)\\ &= (-1)^M\left[n_0\sum_{jkl} q_j^{2\mu+2\omega}q_k^{2\nu}q_l^{2M-2\mu-2\nu-2\omega-2\kappa-2\tau}(\mathbf{q}_j\cdot\mathbf{q}_k)^{\kappa}(\mathbf{q}_j\cdot\mathbf{q}_l)^{\tau}A_jA_kA_l\delta_{\mathbf{q}_j+\mathbf{q}_k+\mathbf{q}_l,0}\right.\\ &\qquad\left.+\sum_{ijkl}|\mathbf{q}_i+\mathbf{q}_j|^{2\mu}q_j^{2\omega}q_k^{2\nu}q_l^{2M-2\mu-2\nu-2\omega-2\kappa-2\tau}(\mathbf{q}_j\cdot\mathbf{q}_k)^{\kappa}(\mathbf{q}_j\cdot\mathbf{q}_l)^{\tau}A_iA_jA_kA_l\delta_{\mathbf{q}_i+\mathbf{q}_j+\mathbf{q}_k+\mathbf{q}_l,0}\right],\end{aligned} \tag{S21}$$

$$\begin{aligned}&\frac{1}{V}\int d\mathbf{r}n\sum_{\alpha_{i'},\beta_{j'},\gamma_{k'}=x,y,z}\;\sum_{\alpha,\beta,\gamma=x,y,z}\epsilon_{\alpha\beta\gamma}\left(\nabla^{2\mu}\prod_{i'=1}^{\kappa}\prod_{k'=1}^{\lambda}\partial_{\alpha_{i'}}\partial_{\gamma_{k'}}\partial_{\alpha}n\right)\\ &\qquad\times\left(\nabla^{2\nu}\prod_{i'=1}^{\kappa}\prod_{j'=1}^{\tau}\partial_{\alpha_{i'}}\partial_{\beta_{j'}}\partial_{\beta}n\right)\left(\nabla^{2\omega}\prod_{j'=1}^{\tau}\prod_{k'=1}^{\lambda}\partial_{\beta_{j'}}\partial_{\gamma_{k'}}\partial_{\gamma}n\right)\\ &= (-1)^{\mu+\nu+\omega+\kappa+\tau+\lambda}\sum_{ijkl}\left[(\mathbf{q}_j\times\mathbf{q}_k)\cdot\mathbf{q}_l\right]q_j^{2\mu}q_k^{2\nu}q_l^{2\omega}(\mathbf{q}_j\cdot\mathbf{q}_k)^{\kappa}(\mathbf{q}_k\cdot\mathbf{q}_l)^{\tau}(\mathbf{q}_j\cdot\mathbf{q}_l)^{\lambda}A_iA_jA_kA_l\delta_{\mathbf{q}_i+\mathbf{q}_j+\mathbf{q}_k+\mathbf{q}_l,0}.\end{aligned} \tag{S22}$$

In Eqs. (S20) and (S21), the angle dependence arises from $|\mathbf{q}_i+\mathbf{q}_j|^{2\mu}$, with $\mu\geq2$ for pairwise resonant wavevectors $\mathbf{q}_i-\mathbf{q}_i+\mathbf{q}_j-\mathbf{q}_j=0$ (see below) and $\mu\geq1$ for nonpairwise wavevector closed loops, and also from $(\mathbf{q}_j\cdot\mathbf{q}_k)^{\kappa}$, $(\mathbf{q}_j\cdot\mathbf{q}_l)^{\tau}$ in fourth-order expansion terms. There is no angle dependence in 3rd-order expansion terms of Eqs. (S20) and (S21), due to $\mathbf{q}_j\cdot\mathbf{q}_k=(q_l^2-q_j^2-q_k^2)/2$ as a result of $\mathbf{q}_j+\mathbf{q}_k+\mathbf{q}_l=0$. The result of Eq. (S22) is independent of average density $n_0$ and has no 3rd-order contribution. It is nonzero only for nonpairwise wavevectors, and is equal to 0 for any pairwise resonant wavevector tetrads, for which two of $\mathbf{q}_j$, $\mathbf{q}_k$, and $\mathbf{q}_l$ are always parallel or anti-parallel to each other, leading to $(\mathbf{q}_j\times\mathbf{q}_k)\cdot\mathbf{q}_l=0$.

Note that the above derivation process is generic, and can be applied to any order of direct correlation function $C^{(m)}$ (e.g., 5-point, 6-point, etc.) based on Eq. (S3).

## II. ANALYSIS OF ANGLE DEPENDENCE AND CONTROL FOR $\hat{C}^{(4)}$ CONTRIBUTIONS

To identify the effects of angle dependence from $\Delta\mathcal{F}^{(4)}$ terms, we need to consider the wavevector resonant condition $\mathbf{q}_i+\mathbf{q}_j+\mathbf{q}_k+\mathbf{q}_l=0$, including 3 types of closed-loop combinations [6, 7]: collinear, pairwise, and nonpairwise.

### Collinear wavevectors $\mathbf{q}_i - \mathbf{q}_i + \mathbf{q}_i - \mathbf{q}_i = 0$

Given $n_q$ wavevectors $\mathbf{q}_1$, $\mathbf{q}_2$, ..., $\mathbf{q}_{n_q}$, there are totally $6n_q$ collinear combinations, but only $2n_q$ of them give $|\mathbf{q}_i + \mathbf{q}_i| \neq 0$. The corresponding results for the last term of Eqs. (S20) and (S21) are angle independent, i.e.,

$$f^C = c(-1)^M 2^{2\mu+1} \sum_{j=1}^{n_q} q_j^{2M} |A_j|^4, \tag{S23}$$

with $c = 1$ for Eq. (S20) and $c = (-1)^{\kappa+\tau}$ for Eq. (S21). The collinear result for Eq. (S22) is 0.

### Pairwise wavevector closed loops $\mathbf{q}_i - \mathbf{q}_i + \mathbf{q}_j - \mathbf{q}_j = 0$

There are totally $12n_q(n_q - 1)$ non-collinear pairwise combinations of wavevector loops, and $8n_q(n_q - 1)$ of them give nonzero $|\mathbf{q}_i + \mathbf{q}_j|$. For any pair of wavevectors $(\mathbf{q}_i, \mathbf{q}_j)$ with $i, j = 1, 2, ..., n_q$, $i \neq j$, $q_j = \gamma q_i \equiv \gamma q$, and angle $\theta$ between $\mathbf{q}_i$ and $\mathbf{q}_j$, from Eqs. (S20) and (S21) we have (noting $A_{-j}(-\mathbf{q}_j) = A_j^*(\mathbf{q}_j)$)

$$\begin{aligned}
&\frac{1}{V}\int d\mathbf{r} \left[\nabla^{2\mu}(n\nabla^{2\omega}n)\right] (\nabla^{2\nu}n)(\nabla^{2M-2\mu-2\nu-2\omega}n)\Big|_{n_0=0}^{(P)} \\
&= (-1)^M 2 \left(|\mathbf{q}_i + \mathbf{q}_j|^{2\mu} + |\mathbf{q}_i - \mathbf{q}_j|^{2\mu}\right) \left(q_i^{2\nu} q_j^{2M-2\mu-2\nu-2\omega} + q_i^{2M-2\mu-2\nu-2\omega} q_j^{2\nu}\right) \left(q_i^{2\omega} + q_j^{2\omega}\right) |A_i|^2 |A_j|^2 \\
&= (-1)^M 2q^{2M} \left[(1 + \gamma^2 + 2\gamma\cos\theta)^\mu + (1 + \gamma^2 - 2\gamma\cos\theta)^\mu\right] (\gamma^{2M-2\mu-2\nu-2\omega} + \gamma^{2\nu})(1 + \gamma^{2\omega})|A_i|^2|A_j|^2,
\end{aligned} \tag{S24}$$

$$\begin{aligned}
&\frac{1}{V}\int d\mathbf{r} \sum_{\alpha_{i'}\beta_{j'}} \left[\nabla^{2\mu}\left(n\nabla^{2\omega}\prod_{i'=1}^{\kappa}\prod_{j'=1}^{\tau}\partial_{\alpha_{i'}}\partial_{\beta_{j'}}n\right)\right] \left(\nabla^{2\nu}\prod_{i'=1}^{\kappa}\partial_{\alpha_{i'}}n\right) \left(\nabla^{2\eta}\prod_{j'=1}^{\tau}\partial_{\beta_{j'}}n\right)\Bigg|_{n_0=0}^{(P)} \\
&= (-1)^M 2 \Big\{ \left[(-1)^\kappa|\mathbf{q}_i + \mathbf{q}_j|^{2\mu} + |\mathbf{q}_i - \mathbf{q}_j|^{2\mu}\right] (-1)^\tau (\mathbf{q}_i \cdot \mathbf{q}_j)^\kappa \left(q_i^{2\nu} q_j^{2\omega+2\tau+2\eta} + q_i^{2\omega+2\tau+2\eta} q_j^{2\nu}\right) \\
&\qquad + \left[(-1)^\tau|\mathbf{q}_i + \mathbf{q}_j|^{2\mu} + |\mathbf{q}_i - \mathbf{q}_j|^{2\mu}\right] (-1)^\kappa (\mathbf{q}_i \cdot \mathbf{q}_j)^\tau \left(q_i^{2\eta} q_j^{2\omega+2\nu+2\kappa} + q_i^{2\omega+2\nu+2\kappa} q_j^{2\eta}\right) \Big\} |A_i|^2|A_j|^2 \\
&= (-1)^{M+\kappa+\tau} 2q^{2M} \Big\{ \left[(1 + \gamma^2 + 2\gamma\cos\theta)^\mu + (1 + \gamma^2 - 2\gamma\cos\theta)^\mu (-1)^\kappa\right] \cos^\kappa\theta \, \gamma^\kappa (\gamma^{2\omega+2\tau+2\eta} + \gamma^{2\nu}) \\
&\qquad + \left[(1 + \gamma^2 + 2\gamma\cos\theta)^\mu + (1 + \gamma^2 - 2\gamma\cos\theta)^\mu (-1)^\tau\right] \cos^\tau\theta \, \gamma^\tau (\gamma^{2\omega+2\nu+2\kappa} + \gamma^{2\eta}) \Big\} |A_i|^2|A_j|^2,
\end{aligned} \tag{S25}$$

where $\eta = M - \mu - \nu - \omega - \kappa - \tau$. The result of Eq. (S22) is 0 for pairwise wavevectors.

When minimizing the above pairwise contributions with respect to $\theta$, one of the solutions is $\sin\theta = 0$, giving $\theta = 0$ or $\pi$ (i.e., the stripe phase). The other solution is $\cos\theta = 0$ and thus $\theta_{\min} = \pm\pi/2$, which would correspond to the minimum free energy contribution if $\mu \geq 2$ and $(-1)^M > 0$ for Eq. (S24). The same result of $\theta_{\min} = \pm\pi/2$ can be also obtained for Eq. (S25), when i) $\mu \geq 1$ and at least one of $\kappa, \tau \geq 1$, or ii) $\mu = 0$ and at least one of $\kappa, \tau \geq 2$. Thus, any single angle-dependent gradient term of $\hat{C}^{(4)}$ free energy contribution will always lead to a $\pi/2$ pattern angle if considering only pairwise wavevectors and the same angle $\theta$ between any two wavevectors $\mathbf{q}_i$ and $\mathbf{q}_j$.

To obtain other angle values and be able to achieve angle control or tuning of the crystalline structure, we need to use the combination of different nonlinear gradient terms such as $\sum_k E_k n(\nabla^{2\mu_k} n^2)(\nabla^{2M_k - 2\mu_k} n)$ with $M_k \geq \mu_k$, via choosing coefficients $E_k$ based on the desired value of $\theta_{\min}$. The corresponding analysis and results are given in the main text.

### Nonpairwise wavevector tetrads $\mathbf{q}_i + \mathbf{q}_j + \mathbf{q}_k + \mathbf{q}_l = 0$

If there are $m_q = m_{q3} + m_{q2} + m_{q1}$ distinct nonpairwise loops among $n_q$ wavevectors $\mathbf{q}_1$, $\mathbf{q}_2$, ..., $\mathbf{q}_{n_q}$, we have (i) $8m_{q3}$ combinations if $i = j = k \neq l$, for $m_{q3}$ distinct loops of $3\mathbf{q}_i + \mathbf{q}_l = 0$ among those $n_q$ wavevectors; (ii) $24m_{q2}$ combinations if $i = j \neq k \neq l$, for $m_{q2}$ distinct loops of $2\mathbf{q}_i + \mathbf{q}_k + \mathbf{q}_l = 0$; (iii) $48m_{q1}$ combinations if $i \neq j \neq k \neq l$, for $m_{q1}$ distinct loops of $\mathbf{q}_i + \mathbf{q}_j + \mathbf{q}_k + \mathbf{q}_l = 0$ (e.g., $m_{q1} = 1$, $m_{q2} = m_{q3} = 0$ for the first mode of 3D fcc or diamond cubic phase with 4 wavevectors $\mathbf{q}_1 + \mathbf{q}_2 + \mathbf{q}_3 + \mathbf{q}_4 = 0$). The angle dependence would then always occur for the $C^{(4)}$ gradient terms containing $\nabla^{2\mu}n^2$ ($\mu \geq 1$). For the example of 1st-mode fcc or diamond cubic phase with

amplitude $A_j = |A|e^{i\phi_j}$, $\mathbf{q}_1 = q(-1,1,1)/\sqrt{3}$, $\mathbf{q}_2 = q(1,-1,1)/\sqrt{3}$, $\mathbf{q}_3 = q(1,1,-1)/\sqrt{3}$, and $\mathbf{q}_4 = q(-1,-1,-1)/\sqrt{3}$; the corresponding nonpairwise contribution to $[\nabla^{2\mu}(n\nabla^{2\omega}n)](\nabla^{2\nu}n)(\nabla^{2M-2\mu-2\nu-2\omega}n)$ is given by

$$\frac{1}{V}\int d\mathbf{r}\left[\nabla^{2\mu}(n\nabla^{2\omega}n)\right](\nabla^{2\nu}n)(\nabla^{2M-2\mu-2\nu-2\omega}n)\Big|_{n_0=0}^{(NP)}$$
$$= (-1)^M 48q^{2M}2^{\mu}\cos(\phi_1+\phi_2+\phi_3+\phi_4)(1+\cos\theta)^{\mu}|A|^4 = \pm(-1)^M 48q^{2M}2^{\mu}(1+\cos\theta)^{\mu}|A|^4, \tag{S26}$$

with "+" for fcc of phases $\phi_j = 0$ and "−" for diamond cubic of phases $\phi_j = \pi/4$ $(j = 1,2,3,4)$.

## III. ANGLE DEPENDENCE OF $\hat{C}^{(3)}$ INFINITE SERIES EXPANSION

There are two angle-dependent PFC models developed very recently [2, 3], using three-point direction correlation $C^{(3)}$ and the separation of its radial and angular dependence that satisfies the condition of rotational invariance. In the following we show that the $\hat{C}^{(3)}$ form adapted in Ref. [2] can be mapped to the general form of Eq. (S6) determined by the property of isotropic tensors, as an infinite series expansion, while a similar mapping could be obtained for the model of Ref. [3] under some special conditions.

(i) In the 2D XPFC model of Ref. [2], $C^{(3)}$ is assumed as

$$C^{(3)}(\mathbf{r}_1-\mathbf{r}_2,\mathbf{r}_1-\mathbf{r}_3) = \sum_{i=1}^{2} C_s^{(i)}(\mathbf{r}_1-\mathbf{r}_2)C_s^{(i)}(\mathbf{r}_1-\mathbf{r}_3) = C_s^{(1)}(\mathbf{r})C_s^{(1)}(\mathbf{r}') + C_s^{(2)}(\mathbf{r})C_s^{(2)}(\mathbf{r}'), \tag{S27}$$

where $\mathbf{r} \equiv \mathbf{r}_1-\mathbf{r}_2$, $\mathbf{r}' \equiv \mathbf{r}_1-\mathbf{r}_3$, and in 2D polar coordinate $(r,\theta)$,

$$C_s^{(1)}(r,\theta) = C_r(r)\cos(m\theta), \quad C_s^{(2)}(r,\theta) = C_r(r)\sin(m\theta), \quad C_r(r) = \frac{X}{2\pi a_0}\delta(r-a_0), \tag{S28}$$

with $a_0$ the lattice spacing and $X$ a constant. It has been proved in Ref. [2] that this approximation of $C^{(3)}$ gives both angle dependence and rotational invariance, with

$$C^{(3)}(\mathbf{r},\mathbf{r}') = C_r(r)C_r(r')\cos[m(\theta-\theta')] = \left(\frac{X}{2\pi a_0}\right)^2 \delta(r-a_0)\delta(r'-a_0)\cos[m(\theta-\theta')]. \tag{S29}$$

From Eq. (S27) the Fourier transform of $C^{(3)}$ can be expressed as

$$\hat{C}^{(3)}(\mathbf{q}_1,\mathbf{q}_2) = \sum_{i=1}^{2}\hat{C}_s^{(i)}(\mathbf{q}_1)\hat{C}_s^{(i)}(\mathbf{q}_2), \tag{S30}$$

(note that there is no convolution here due to the separation of $\mathbf{r}$ and $\mathbf{r}'$ in $C^{(3)}$), where

$$\hat{C}_s^{(1)}(\mathbf{q}) = \hat{C}_s^{(1)}(q,\theta_q) = Xi^m\cos(m\theta_q)J_m(qa_0), \quad \hat{C}_s^{(2)}(\mathbf{q}) = \hat{C}_s^{(2)}(q,\theta_q) = Xi^m\sin(m\theta_q)J_m(qa_0), \tag{S31}$$

are the Fourier transform of $C_s^{(1)}(r,\theta)$ and $C_s^{(2)}(r,\theta)$ [2]. Here $J_m(qa_0)$ is the Bessel function of the 1st kind, and can be expressed as an infinite power series of $q$, i.e.,

$$J_m(qa_0) = \sum_{k=0}^{\infty}\frac{(-1)^k}{k!\Gamma(k+m+1)}\left(\frac{qa_0}{2}\right)^{2k+m} = q^m\sum_{k=0}^{\infty}\alpha_k q^{2k}, \tag{S32}$$

where $\alpha_k = \frac{(-1)^k}{k!\Gamma(k+m+1)}(a_0/2)^{2k+m}$. Thus

$$\hat{C}^{(3)}(\mathbf{q}_1,\mathbf{q}_2) = (Xi^m)^2 J_m(q_1a_0)J_m(q_2a_0)\left[\cos(m\theta_{q_1})\cos(m\theta_{q_2}) + \sin(m\theta_{q_1})\sin(m\theta_{q_2})\right]$$
$$= -X^2\sum_{j,k=0}^{\infty}\alpha_j\alpha_k q_1^{2j}q_2^{2k}q_1^m q_2^m\cos(m\theta_{12}), \tag{S33}$$

with $\theta_{12} = \theta_{q_1} - \theta_{q_2}$, showing the rotational invariance in Fourier space.

Noting that

$$\cos(m\theta) = T_m(\cos\theta) = \frac{m}{2}\sum_{k=0}^{[m/2]} \frac{(-1)^k}{m-k}\binom{m-k}{k}(2\cos\theta)^{m-2k} \equiv \sum_{k=0}^{[m/2]} \beta_k (\cos\theta)^{m-2k}, \tag{S34}$$

where $T_m$ are the Chebyshev polynomials and $\beta_k = \frac{m}{2}\frac{(-1)^k}{m-k}\binom{m-k}{k}2^{m-2k}$, we have

$$\hat{C}^{(3)}(\mathbf{q}_1, \mathbf{q}_2) = -X^2 \left( \sum_{j,k=0}^{\infty} \alpha_j \alpha_k q_1^{2j} q_2^{2k} \right) \sum_{l=0}^{[m/2]} \beta_l q_1^{2l} q_2^{2l} (\mathbf{q}_1 \cdot \mathbf{q}_2)^{m-2l} \equiv \hat{C}^{(3)}(q_1^2, q_2^2, \mathbf{q}_1 \cdot \mathbf{q}_2), \tag{S35}$$

which is an infinite series of $q_1^2$, $q_2^2$, $\mathbf{q}_1 \cdot \mathbf{q}_2$ that satisfies the condition of isotropic tensors and the general expansion form of Eq. (S6). Note also that the corresponding real-space function $C^{(3)}$ involves Dirac delta functions as shown in Eq. (S29).

(ii) In the PFC model of Ref. [3], the expansion form of $\hat{C}^{(3)}$ is assumed to be

$$\hat{C}^{(3)}(\mathbf{q}_1, \mathbf{q}_2) = \beta^2 R(q_1) R(q_2) \sum_{l=0}^{l_{\max}} \alpha_l P_l(\hat{q}_1 \cdot \hat{q}_2), \tag{S36}$$

where $\beta$, $\alpha_l$ are constants, $R(q)$ is a radial function, and $P_l$ are the Legendre polynomials given by

$$P_l(\hat{q}_1 \cdot \hat{q}_2) = \frac{1}{2^l}\sum_{k=0}^{[l/2]} (-1)^k \binom{l}{k}\binom{2l-2k}{l} (\hat{q}_1 \cdot \hat{q}_2)^{l-2k} \equiv \sum_{k=0}^{[l/2]} \gamma_{kl} (\hat{q}_1 \cdot \hat{q}_2)^{l-2k}, \tag{S37}$$

where $\gamma_{kl} = \frac{(-1)^k}{2^l}\binom{l}{k}\binom{2l-2k}{l}$. If assuming $R(q)$ as a power series, i.e., $R(q) = \sum_{j=j0}^{\infty} R_j q^j$, we get

$$\begin{aligned}
\hat{C}^{(3)}(\mathbf{q}_1, \mathbf{q}_2) &= \beta^2 \sum_{l=0}^{l_{\max}} \sum_{k=0}^{[l/2]} \sum_{j_1, j_2 = j_0}^{\infty} R_{j_1} R_{j_2} \alpha_l \gamma_{kl} q_1^{j_1} q_2^{j_2} (\hat{q}_1 \cdot \hat{q}_2)^{l-2k} \\
&= \beta^2 \sum_{l=0}^{l_{\max}} \sum_{k=0}^{[l/2]} \sum_{j_1, j_2 = j_0}^{\infty} R_{j_1} R_{j_2} \alpha_l \gamma_{kl} q_1^{j_1 - l + 2k} q_2^{j_2 - l + 2k} (\mathbf{q}_1 \cdot \mathbf{q}_2)^{l-2k}.
\end{aligned} \tag{S38}$$

Thus only in the condition that $j_1 - l + 2k = 2m_1 \geq 0$ and $j_2 - l + 2k = 2m_2 \geq 0$, which requires $j_1 = l + 2m_{j_1}$ and $j_2 = l + 2m_{j_2}$ with $m_{j_1}, m_{j_2} = 0, 1, 2, ...$ (i.e., $j_1$, $j_2$, and $l$ are all even or all odd and $j_0 \geq l$, making $R(q)$ $l$-dependent), we can reproduce the form $\hat{C}^{(3)} = \hat{C}^{(3)}(q_1^2, q_2^2, \mathbf{q}_1 \cdot \mathbf{q}_2)$ as that of Eq. (S6). Note that this condition is not satisfied for the choice of $R(q) = A_2 \exp[-(q - q_0)^2 / 2\sigma^2]$ used in Ref. [3].

* liuzhirong@pku.edu.cn
† huang@wayne.edu

[1] H. Jeffreys, Proc. Camb. Phil. Soc. **73**, 173 (1973); P. G. Appleby, B. R. Duffy, and R. W. Ogden, Glasgow Math. J. **29**, 185 (1987); E. A. Kearsley and J. T. Fong, J. Res. Nat. Bur. Stand. **79B**, 49 (1975).
[2] M. Seymour and N. Provatas, Phys. Rev. B **93**, 035447 (2016).
[3] E. Alster, D. Montiel, K. Thornton, and P. W. Voorhees, Phys. Rev. Materials **1**, 060801 (2017).
[4] M. Bestehorn and C. Pérez-García, Physica D **61**, 67 (1992).
[5] M. R. E. Proctor, J. Fluid Mech. **113**, 469 (1981); V. L. Gertsberg and G. I. Sivashinsky, Prog. Theor. Phys. **66**, 1219 (1981).
[6] J. L. Jones and M. Olvera de la Cruz, J. Chem. Phys. **100**, 5272 (1994).
[7] S. K. Mkhonta, K. R. Elder, and Z.-F. Huang, Phys. Rev. Lett. **116**, 205502 (2016).
